# Supplementary material for: Improved Benthic Classification using Resolution Scaling and SymmNet Unsupervised Domain Adaptation
Source: arXiv:2303.10960 source file (2023-03-20)
Supplement: Supplementary file 1 [file additional.tex]

\section{Method}
SHOT
Uses only target data to improve data
Information maximisation loss using entropy and ???
Self-supervised learning using pseudo labels based on distance to centroid of each class.
Ignored rotation based semi-supervised pretext task as these images are rotation invariant.

Also tried MixMatch a semi-supervised method in  a self-supervised way.  Data is split into labelled and unlabelled based on an entropy measure to split the samples with higher probability of being correct.  MixMatch then uses a stochastic based augmentation of labelled and unlabelled data to train the model further.

\section{Results and Discussion}
UDA is usually based on source with large number of samples and target with smaller number of samples??
